# Supplementary material for: TSMixer: Lightweight MLP-Mixer Model for Multivariate Time Series Forecasting
Source: arXiv:2306.09364 source file (2023-12-11)
Supplement: Supplementary file 1 [file appendix.tex]

\section{Appendix}

\subsection{Experiments}



\begin{table*}
\centering
\setlength{\tabcolsep}{2pt}
\scalebox{1.1}{
\begin{tabular}{c|c|c|c|c}
\hline  
Data & \makecell{FL} & \makecell{\textbf{\citsm-Best}}  & LightTS & S4  \\
\hline
\multirow{2}{*}{ETTH1} & 336 & \textbf{0.421} & 0.466 & 1.407  \\ 
& 720 & \textbf{0.444}  & 0.542 & 1.162 \\ \hline
\multirow{2}{*}{ETTH2} & 336 & \textbf{0.357} & 0.497 & 1.98  \\ 
& 720 & \textbf{0.395} & 0.739 & 2.65  \\ \hline
\multirow{2}{*}{Weather} & 336 & \textbf{0.243} & 0.527 & 0.531  \\ 
& 720 & \textbf{0.316} & 0.554 & 0.578  \\ \hline
\multicolumn{3}{c|}{\makecell{\textbf{\citsm-Best \% improvement }}}& \textbf{33.2\%} & \textbf{66.4\%} \\ \hline
\end{tabular}}
\caption{LightTS and S4 MSE Benchmarking}
\label{tab:lightts}
\end{table*}


\begin{table*}[t]
        % \small
	\centering
	\resizebox{\linewidth}{!}{
		\begin{tabular}{cc|c|cc|cc|cc|cc|ccc}
			\cline{2-13}
			&\multicolumn{2}{c|}{Models}& \multicolumn{2}{c|}{PatchTST}& \multicolumn{2}{c|}{DLinear}& \multicolumn{2}{c|}{\citsm(\ga,\hr)}& \multicolumn{2}{c|}{\citsm(\ga,\hr,\cc)}& \multicolumn{2}{c}{\citsm-Best} \\
			\cline{2-13}
			&\multicolumn{2}{c|}{Metric}&MSE&MAE&MSE&MAE&MSE&MAE&MSE&MAE&MSE&MAE\\
			\cline{2-13}
        
            &\multirow{4}*{\rotatebox{90}{ETTH1}} & 96 & \uline{0.37} & 0.4 & 0.375 & \uline{0.399} & \textbf{0.368} & \textbf{0.398} & \textbf{0.368} & \textbf{0.398} & \textbf{0.368} & \textbf{0.398} \\ 
            &\multicolumn{1}{c|}{} & 192 & 0.413 & 0.429 & 0.405 & \textbf{0.416} & \textbf{0.399} & \uline{0.418} & \uline{0.4} & \uline{0.418} & \textbf{0.399} & \uline{0.418} \\ 
            &\multicolumn{1}{c|}{} & 336 & \uline{0.422} & 0.44 & 0.439 & 0.443 & \textbf{0.421} & \textbf{0.436} & \uline{0.422} & \uline{0.437} & \textbf{0.421} & \textbf{0.436} \\ 
            &\multicolumn{1}{c|}{} & 720 & \uline{0.447} & \uline{0.468} & 0.472 & 0.49 & \textbf{0.444} & \textbf{0.467} & 0.45 & \textbf{0.467} & \textbf{0.444} & \textbf{0.467} \\ 
            \cline{2-13} 
            &\multirow{4}*{\rotatebox{90}{ETTH2}} & 96 & \textbf{0.274} & \textbf{0.337} & 0.289 & 0.353 & \uline{0.276} & \textbf{0.337} & \uline{0.276} & \uline{0.339} & \uline{0.276} & \textbf{0.337} \\ 
            &\multicolumn{1}{c|}{} & 192 & 0.341 & 0.382 & 0.383 & 0.418 & \uline{0.335} & \uline{0.377} & \textbf{0.33} & \textbf{0.374} & \textbf{0.33} & \textbf{0.374} \\ 
            &\multicolumn{1}{c|}{} & 336 & \textbf{0.329} & \textbf{0.384} & 0.448 & 0.465 & 0.369 & 0.406 & \uline{0.357} & \uline{0.401} & \uline{0.357} & \uline{0.401} \\ 
            &\multicolumn{1}{c|}{} & 720 & \textbf{0.379} & \textbf{0.422} & 0.605 & 0.551 & 0.409 & 0.447 & \uline{0.395} & \uline{0.436} & \uline{0.395} & \uline{0.436} \\ 
            \cline{2-13} 
            &\multirow{4}*{\rotatebox{90}{ETTM1}} & 96 & \uline{0.293} & \uline{0.346} & 0.299 & \textbf{0.343} & 0.297 & 0.348 & \textbf{0.291} & \uline{0.346} & \textbf{0.291} & \uline{0.346} \\ 
            &\multicolumn{1}{c|}{} & 192 & \textbf{0.333} & 0.37 & 0.335 & \textbf{0.365} & \textbf{0.333} & \uline{0.369} & \uline{0.334} & \uline{0.369} & \textbf{0.333} & \uline{0.369} \\ 
            &\multicolumn{1}{c|}{} & 336 & 0.369 & 0.392 & 0.369 & \uline{0.386} & \textbf{0.365} & \textbf{0.385} & \uline{0.367} & 0.387 & \textbf{0.365} & \textbf{0.385} \\ 
            &\multicolumn{1}{c|}{} & 720 & \textbf{0.416} & 0.42 & 0.425 & 0.421 & \textbf{0.416} & \textbf{0.413} & \uline{0.421} & \uline{0.415} & \textbf{0.416} & \textbf{0.413} \\ 
            \cline{2-13} 
            &\multirow{4}*{\rotatebox{90}{ETTM2}} & 96 & 0.166 & \uline{0.256} & 0.167 & 0.26 & \textbf{0.164} & \textbf{0.255} & \uline{0.165} & \textbf{0.255} & \textbf{0.164} & \textbf{0.255} \\ 
            &\multicolumn{1}{c|}{} & 192 & \uline{0.223} & \uline{0.296} & 0.224 & 0.303 & \textbf{0.219} & \textbf{0.293} & 0.225 & 0.299 & \textbf{0.219} & \textbf{0.293} \\ 
            &\multicolumn{1}{c|}{} & 336 & \uline{0.274} & \textbf{0.329} & 0.281 & 0.342 & \textbf{0.273} & \uline{0.33} & \textbf{0.273} & \textbf{0.329} & \textbf{0.273} & \textbf{0.329} \\ 
            &\multicolumn{1}{c|}{} & 720 & 0.362 & 0.385 & 0.397 & 0.421 & \textbf{0.358} & \textbf{0.38} & \uline{0.361} & \uline{0.383} & \textbf{0.358} & \textbf{0.38} \\ 
            \cline{2-13} 
            &\multirow{4}*{\rotatebox{90}{Electricity}} & 96 & \textbf{0.129} & \textbf{0.222} & \uline{0.14} & 0.237 & \textbf{0.129} & \uline{0.224} & \textbf{0.129} & 0.225 & \textbf{0.129} & \uline{0.224} \\ 
            &\multicolumn{1}{c|}{} & 192 & \uline{0.147} & \textbf{0.24} & 0.153 & 0.249 & 0.148 & \uline{0.242} & \textbf{0.146} & \uline{0.242} & \textbf{0.146} & \uline{0.242} \\ 
            &\multicolumn{1}{c|}{} & 336 & \uline{0.163} & \uline{0.259} & 0.169 & 0.267 & 0.164 & \uline{0.259} & \textbf{0.158} & \textbf{0.256} & \textbf{0.158} & \textbf{0.256} \\ 
            &\multicolumn{1}{c|}{} & 720 & \uline{0.197} & \uline{0.29} & 0.203 & 0.301 & 0.201 & 0.292 & \textbf{0.186} & \textbf{0.282} & \textbf{0.186} & \textbf{0.282} \\ 
            \cline{2-13} 
            &\multirow{4}*{\rotatebox{90}{Traffic}} & 96 & \uline{0.36} & \uline{0.249} & 0.41 & 0.282 & \textbf{0.356} & \textbf{0.248} & 0.369 & 0.264 & \textbf{0.356} & \textbf{0.248} \\ 
            &\multicolumn{1}{c|}{} & 192 & \uline{0.379} & \textbf{0.256} & 0.423 & 0.287 & \textbf{0.377} & \uline{0.257} & 0.393 & 0.278 & \textbf{0.377} & \uline{0.257} \\ 
            &\multicolumn{1}{c|}{} & 336 & \uline{0.392} & \uline{0.264} & 0.436 & 0.296 & \textbf{0.385} & \textbf{0.262} & 0.406 & 0.285 & \textbf{0.385} & \textbf{0.262} \\ 
            &\multicolumn{1}{c|}{} & 720 & \uline{0.432} & \uline{0.286} & 0.466 & 0.315 & \textbf{0.424} & \textbf{0.283} & 0.445 & 0.304 & \textbf{0.424} & \textbf{0.283} \\ 
            \cline{2-13} 
            &\multirow{4}*{\rotatebox{90}{Weather}} & 96 & 0.149 & \uline{0.198} & 0.176 & 0.237 & \uline{0.148} & \uline{0.198} & \textbf{0.146} & \textbf{0.197} & \textbf{0.146} & \textbf{0.197} \\ 
            &\multicolumn{1}{c|}{} & 192 & 0.194 & \uline{0.241} & 0.22 & 0.282 & \uline{0.193} & \textbf{0.24} & \textbf{0.191} & \textbf{0.24} & \textbf{0.191} & \textbf{0.24} \\ 
            &\multicolumn{1}{c|}{} & 336 & 0.245 & 0.282 & 0.265 & 0.319 & \textbf{0.243} & \textbf{0.279} & \uline{0.244} & \uline{0.28} & \textbf{0.243} & \textbf{0.279} \\ 
            &\multicolumn{1}{c|}{} & 720 & \textbf{0.314} & \uline{0.334} & 0.323 & 0.362 & 0.317 & \textbf{0.333} & \uline{0.316} & \textbf{0.333} & \uline{0.316} & \textbf{0.333} \\ 
            \cline{2-13} 
		\end{tabular}
	}
	\caption{\citsm-Best Drill-down}
	\label{tab:supervised-ab1}
\end{table*}




\begin{table*}[t]
        % \small
	\centering
	\resizebox{\linewidth}{!}{
		\begin{tabular}{cc|c|cc|cc|cc|cc|ccc}
			\cline{2-13}
			&\multicolumn{2}{c|}{Models}& \multicolumn{2}{c|}{V-\tsm}& \multicolumn{2}{c|}{CI-\tsm}& \multicolumn{2}{c|}{\citsm(\ga)}& \multicolumn{2}{c|}{\citsm(\hr)}& \multicolumn{2}{c}{\citsm(\ga,\hr)} \\
			\cline{2-13}
			&\multicolumn{2}{c|}{Metric}&MSE&MAE&MSE&MAE&MSE&MAE&MSE&MAE&MSE&MAE\\
			\cline{2-13}
        &\multirow{4}*{\rotatebox{90}{ETTH1}} & 96.0 & 0.449 & 0.462 & \uline{0.375} & 0.401 & \uline{0.375} & \uline{0.4} & 0.377 & 0.405 & \textbf{0.368} & \textbf{0.398} \\ 
        &\multicolumn{1}{c|}{} & 192.0 & 0.485 & 0.484 & 0.411 & 0.426 & \uline{0.408} & \uline{0.422} & 0.41 & 0.428 & \textbf{0.399} & \textbf{0.418} \\ 
        &\multicolumn{1}{c|}{} & 336.0 & 0.504 & 0.497 & 0.437 & 0.445 & 0.433 & \uline{0.439} & \uline{0.431} & 0.445 & \textbf{0.421} & \textbf{0.436} \\ 
        &\multicolumn{1}{c|}{} & 720.0 & 0.573 & 0.534 & 0.465 & 0.478 & \uline{0.454} & \uline{0.47} & 0.457 & 0.477 & \textbf{0.444} & \textbf{0.467} \\ 
        \cline{2-13} 
        &\multirow{4}*{\rotatebox{90}{ETTH2}} & 96.0 & 0.369 & 0.412 & 0.284 & 0.342 & \textbf{0.276} & \uline{0.339} & \uline{0.283} & 0.341 & \textbf{0.276} & \textbf{0.337} \\ 
        &\multicolumn{1}{c|}{} & 192.0 & 0.391 & 0.428 & 0.353 & 0.384 & \uline{0.338} & \uline{0.379} & 0.344 & 0.38 & \textbf{0.335} & \textbf{0.377} \\ 
        &\multicolumn{1}{c|}{} & 336.0 & 0.403 & 0.44 & \uline{0.365} & \textbf{0.403} & \textbf{0.362} & \uline{0.404} & 0.376 & 0.408 & 0.369 & 0.406 \\ 
        &\multicolumn{1}{c|}{} & 720.0 & 0.475 & 0.481 & \uline{0.406} & \uline{0.442} & 0.415 & 0.451 & \textbf{0.396} & \textbf{0.434} & 0.409 & 0.447 \\ 
        \cline{2-13} 
        &\multirow{4}*{\rotatebox{90}{ETTM1}} & 96.0 & 0.328 & 0.372 & 0.305 & 0.354 & \textbf{0.296} & \uline{0.349} & 0.301 & 0.351 & \uline{0.297} & \textbf{0.348} \\ 
        &\multicolumn{1}{c|}{} & 192.0 & 0.372 & 0.397 & 0.336 & 0.374 & \uline{0.334} & \uline{0.37} & 0.338 & 0.372 & \textbf{0.333} & \textbf{0.369} \\ 
        &\multicolumn{1}{c|}{} & 336.0 & 0.405 & 0.416 & 0.375 & 0.398 & \uline{0.366} & \uline{0.387} & 0.376 & 0.394 & \textbf{0.365} & \textbf{0.385} \\ 
        &\multicolumn{1}{c|}{} & 720.0 & 0.457 & 0.445 & 0.425 & 0.417 & \uline{0.419} & \uline{0.415} & 0.422 & 0.417 & \textbf{0.416} & \textbf{0.413} \\ 
        \cline{2-13} 
        &\multirow{4}*{\rotatebox{90}{ETTM2}} & 96.0 & 0.195 & 0.282 & 0.172 & 0.263 & 0.175 & 0.264 & \uline{0.168} & \uline{0.259} & \textbf{0.164} & \textbf{0.255} \\ 
        &\multicolumn{1}{c|}{} & 192.0 & 0.26 & 0.326 & \uline{0.221} & \uline{0.294} & \uline{0.221} & \uline{0.294} & 0.224 & 0.296 & \textbf{0.219} & \textbf{0.293} \\ 
        &\multicolumn{1}{c|}{} & 336.0 & 0.341 & 0.373 & \textbf{0.273} & \textbf{0.328} & 0.277 & 0.333 & \uline{0.276} & 0.331 & \textbf{0.273} & \uline{0.33} \\ 
        &\multicolumn{1}{c|}{} & 720.0 & 0.437 & 0.432 & \textbf{0.357} & 0.384 & 0.365 & 0.385 & 0.36 & \uline{0.383} & \uline{0.358} & \textbf{0.38} \\ 
        \cline{2-13} 
        &\multirow{4}*{\rotatebox{90}{Electricity}} & 96.0 & 0.212 & 0.323 & \uline{0.13} & \uline{0.224} & \textbf{0.129} & \textbf{0.223} & \uline{0.13} & 0.226 & \textbf{0.129} & \uline{0.224} \\ 
        &\multicolumn{1}{c|}{} & 192.0 & \uline{0.21} & 0.319 & \textbf{0.148} & \uline{0.242} & \textbf{0.148} & \textbf{0.241} & \textbf{0.148} & 0.243 & \textbf{0.148} & \uline{0.242} \\ 
        &\multicolumn{1}{c|}{} & 336.0 & 0.224 & 0.332 & \uline{0.165} & \textbf{0.259} & \uline{0.165} & \textbf{0.259} & \uline{0.165} & \uline{0.26} & \textbf{0.164} & \textbf{0.259} \\ 
        &\multicolumn{1}{c|}{} & 720.0 & 0.251 & 0.352 & \uline{0.204} & 0.293 & \textbf{0.201} & \textbf{0.291} & \uline{0.204} & 0.295 & \textbf{0.201} & \uline{0.292} \\ 
        \cline{2-13} 
        &\multirow{4}*{\rotatebox{90}{Traffic}} & 96.0 & 0.618 & 0.386 & 0.358 & 0.251 & \textbf{0.355} & \textbf{0.246} & 0.357 & 0.251 & \uline{0.356} & \uline{0.248} \\ 
        &\multicolumn{1}{c|}{} & 192.0 & 0.624 & 0.385 & 0.379 & \uline{0.26} & \textbf{0.377} & \textbf{0.257} & \uline{0.378} & \uline{0.26} & \textbf{0.377} & \textbf{0.257} \\ 
        &\multicolumn{1}{c|}{} & 336.0 & 0.63 & 0.38 & 0.388 & 0.265 & \uline{0.387} & \uline{0.264} & \uline{0.387} & 0.265 & \textbf{0.385} & \textbf{0.262} \\ 
        &\multicolumn{1}{c|}{} & 720.0 & 0.66 & 0.389 & 0.426 & 0.286 & 0.427 & \uline{0.285} & \uline{0.425} & 0.286 & \textbf{0.424} & \textbf{0.283} \\ 
        \cline{2-13} 
        &\multirow{4}*{\rotatebox{90}{Weather}} & 96.0 & 0.159 & 0.216 & 0.15 & 0.202 & \uline{0.149} & \uline{0.199} & 0.151 & 0.202 & \textbf{0.148} & \textbf{0.198} \\ 
        &\multicolumn{1}{c|}{} & 192.0 & 0.207 & 0.257 & \uline{0.195} & 0.244 & \uline{0.195} & \uline{0.242} & \uline{0.195} & 0.243 & \textbf{0.193} & \textbf{0.24} \\ 
        &\multicolumn{1}{c|}{} & 336.0 & 0.256 & 0.294 & \uline{0.246} & 0.284 & \uline{0.246} & \uline{0.281} & \uline{0.246} & 0.283 & \textbf{0.243} & \textbf{0.279} \\ 
        &\multicolumn{1}{c|}{} & 720.0 & 0.33 & 0.344 & 0.323 & 0.338 & \textbf{0.317} & \textbf{0.333} & \uline{0.321} & \uline{0.337} & \textbf{0.317} & \textbf{0.333} \\ 
        \cline{2-13} 
        \multicolumn{5}{c|}{ \makecell{\textbf{\% improvement}  \textbf{over \vtsm}}} & \textbf{18\%}	& \textbf{13.8\%} & \textbf{18.5\%} & \textbf{14.3\%}& \textbf{18.1\%} & \textbf{13.9\%} & \textbf{19.3\%} & \textbf{14.8\%} \\ 
            \cline{2-13} 
		\end{tabular}
	}
	\caption{Detail Analysis: Effect of CI, Gated Attention and Hierarchy Reconciliation over Vanilla TSMixer.}
	\label{tab:ga_hc-ab1}
\end{table*}

\begin{table*}[t]
    % \setlength{\tabcolsep}{5pt}
    \centering
    \resizebox{\linewidth}{!}{
    \begin{tabular}{c|c|c|c|c|c|c|c|c|c|c}
        \toprule
        
        \multicolumn{2}{c|}{Models}& V-\tsm & CI-\tsm & IC-\tsm & \multicolumn{6}{c}{\citsm(\ga,\cc)} \\ \hline
        \multicolumn{2}{c|}{Channel Context Length}& \multicolumn{3}{c|}{} & (1) & (2) & (3) & (4) & (5) & (Best) \\ \hline
        \multirow{4}*{\rotatebox{90}{etth1}} & 96.0 & 0.449 & 0.375 & 0.379 & \textbf{0.373} & \textbf{0.373} & 0.377 & \textbf{0.373} & \uline{0.374} & \textbf{0.373} \\ 
        \multicolumn{1}{c|}{} & 192.0 & 0.485 & 0.411 & 0.416 & 0.416 & \textbf{0.407} & \textbf{0.407} & 0.409 & \uline{0.408} & \textbf{0.407} \\ 
        \multicolumn{1}{c|}{} & 336.0 & 0.504 & 0.437 & 0.437 & 0.436 & \uline{0.435} & 0.437 & 0.436 & \textbf{0.43} & \textbf{0.43} \\ 
        \multicolumn{1}{c|}{} & 720.0 & 0.573 & \uline{0.465} & 0.471 & 0.482 & 0.493 & 0.472 & \uline{0.465} & \textbf{0.454} & \textbf{0.454} \\ 
        \hline 
        \multirow{4}*{\rotatebox{90}{etth2}} & 96.0 & 0.369 & 0.284 & 0.291 & \uline{0.27} & 0.274 & 0.277 & 0.275 & \textbf{0.269} & \textbf{0.269} \\ 
        \multicolumn{1}{c|}{} & 192.0 & 0.391 & 0.353 & 0.345 & 0.336 & 0.347 & \uline{0.333} & \textbf{0.33} & 0.339 & \textbf{0.33} \\ 
        \multicolumn{1}{c|}{} & 336.0 & 0.403 & 0.365 & 0.361 & 0.364 & 0.363 & \uline{0.36} & \textbf{0.359} & 0.363 & \textbf{0.359} \\ 
        \multicolumn{1}{c|}{} & 720.0 & 0.475 & 0.406 & 0.419 & 0.4 & \uline{0.398} & 0.41 & \textbf{0.393} & \textbf{0.393} & \textbf{0.393} \\ 
        \hline 
        \multirow{4}*{\rotatebox{90}{ettm1}} & 96.0 & 0.328 & 0.305 & 0.307 & \textbf{0.3} & \uline{0.302} & 0.304 & 0.309 & 0.305 & \textbf{0.3} \\ 
        \multicolumn{1}{c|}{} & 192.0 & 0.372 & \textbf{0.336} & 0.34 & 0.345 & 0.345 & 0.341 & 0.345 & \uline{0.338} & \uline{0.338} \\ 
        \multicolumn{1}{c|}{} & 336.0 & 0.405 & \uline{0.375} & \textbf{0.372} & 0.379 & \uline{0.375} & \uline{0.375} & 0.377 & 0.383 & \uline{0.375} \\ 
        \multicolumn{1}{c|}{} & 720.0 & 0.457 & \uline{0.425} & 0.428 & \textbf{0.422} & 0.426 & 0.429 & 0.426 & 0.44 & \textbf{0.422} \\ 
        \hline 
        \multirow{4}*{\rotatebox{90}{ettm2}} & 96.0 & 0.195 & 0.172 & 0.169 & \uline{0.166} & 0.173 & \textbf{0.165} & \uline{0.166} & 0.168 & \textbf{0.165} \\ 
        \multicolumn{1}{c|}{} & 192.0 & 0.26 & 0.221 & 0.221 & 0.225 & \textbf{0.218} & \uline{0.22} & \uline{0.22} & 0.221 & \textbf{0.218} \\ 
        \multicolumn{1}{c|}{} & 336.0 & 0.341 & \uline{0.273} & 0.278 & \textbf{0.272} & 0.284 & 0.277 & 0.285 & 0.276 & \textbf{0.272} \\ 
        \multicolumn{1}{c|}{} & 720.0 & 0.437 & \textbf{0.357} & 0.367 & 0.359 & \uline{0.358} & 0.385 & 0.362 & 0.362 & \uline{0.358} \\ 
        \hline 
        \multirow{4}*{\rotatebox{90}{electricity}} & 96.0 & 0.212 & \textbf{0.13} & 0.163 & 0.139 & \uline{0.133} & \uline{0.133} & \uline{0.133} & 0.134 & \uline{0.133} \\ 
        \multicolumn{1}{c|}{} & 192.0 & 0.21 & \textbf{0.148} & 0.181 & \uline{0.15} & \uline{0.15} & \uline{0.15} & 0.151 & \uline{0.15} & \uline{0.15} \\ 
        \multicolumn{1}{c|}{} & 336.0 & 0.224 & 0.165 & 0.196 & 0.162 & \textbf{0.159} & \uline{0.161} & \uline{0.161} & 0.163 & \textbf{0.159} \\ 
        \multicolumn{1}{c|}{} & 720.0 & 0.251 & 0.204 & 0.224 & \uline{0.197} & \uline{0.197} & \textbf{0.194} & \textbf{0.194} & \textbf{0.194} & \textbf{0.194} \\ 
        \hline 
        \multirow{4}*{\rotatebox{90}{traffic}} & 96.0 & 0.618 & \textbf{0.358} & 0.468 & 0.382 & 0.384 & 0.384 & \uline{0.374} & 0.387 & \uline{0.374} \\ 
        \multicolumn{1}{c|}{} & 192.0 & 0.624 & \textbf{0.379} & 0.483 & 0.401 & 0.403 & 0.401 & 0.404 & \uline{0.4} & \uline{0.4} \\ 
        \multicolumn{1}{c|}{} & 336.0 & 0.63 & \textbf{0.388} & 0.493 & \uline{0.411} & 0.412 & 0.413 & 0.413 & 0.412 & \uline{0.411} \\ 
        \multicolumn{1}{c|}{} & 720.0 & 0.66 & \textbf{0.426} & 0.524 & 0.448 & 0.457 & \uline{0.445} & 0.454 & 0.451 & \uline{0.445} \\ 
        \hline 
        \multirow{4}*{\rotatebox{90}{weather}} & 96.0 & 0.159 & 0.15 & 0.15 & 0.149 & \textbf{0.146} & 0.148 & \uline{0.147} & 0.15 & \textbf{0.146} \\ 
        \multicolumn{1}{c|}{} & 192.0 & 0.207 & \uline{0.195} & 0.196 & 0.196 & 0.196 & \textbf{0.194} & 0.197 & 0.197 & \textbf{0.194} \\ 
        \multicolumn{1}{c|}{} & 336.0 & 0.256 & \textbf{0.246} & \uline{0.248} & \textbf{0.246} & 0.251 & 0.249 & 0.249 & \textbf{0.246} & \textbf{0.246} \\ 
        \multicolumn{1}{c|}{} & 720.0 & 0.33 & 0.323 & 0.338 & \textbf{0.317} & \uline{0.318} & 0.319 & 0.321 & 0.319 & \textbf{0.317} \\ 
        \hline 
        \multicolumn{3}{c|}{\textbf{\% improvement over \vtsm}}& \textbf{17.9\% }&  \textbf{13.2\%} & \multicolumn{5}{c}{} & \textbf{18.7\%} \\ 
        \hline 
    \end{tabular}
    }
    \caption{Detail Analysis of various Channel Mixing techniques with different context lengths.}
    \label{tab:cc-detail}
\end{table*}

% \begin{table*}[t]
%         \small
% 	\centering
% 	\resizebox{\linewidth}{!}{
% 		\begin{tabular}{c|c|c|c|c|c|c|c|c|c|c}
% 			\hline
% 			&\multicolumn{2}{c|}{Models}& \multicolumn{1}{c|}{V-\tsm}& \multicolumn{1}{c|}{CI-\tsm}& \multicolumn{1}{c|}{IC-\tsm}& \multicolumn{6}{c|}{\citsm(\ga,\cc}\\
% 			\hline
% 			&\multicolumn{2}{c|}{Context Length}&&&&(1)&(2)&(3)&(4)&(5)&(Best)\\
% 			\hline
        
% 		\end{tabular}
% 	}
% 	\caption{Detail Analysis of various Channel Mixing techniques with different context lengths.}
% 	\label{tab:ga_hc-ab1}
% \end{table*}


\begin{table*}
\centering
\setlength{\tabcolsep}{2pt}
\scalebox{1.1}{
\begin{tabular}{c|c|c|c|c|c|c}
\hline  
& \makecell{FL} & \makecell{CI-\tsm\\-Best} & \makecell{CI-\tsm\\(\ga,\hr))} & \makecell{CI-\tsm\\(\ga,\hr,\cc))} & \makecell{PatchTST} & \makecell{BTSF}  \\
\hline
\multirow{5}*{\rotatebox{90}{ETTH1}} & 24 & \textbf{0.314} & \uline{0.319} & \textbf{0.314} & 0.322 & 0.541 \\ 
\multicolumn{1}{c|}{} & 48 & \textbf{0.343} & \uline{0.344} & \textbf{0.343} & 0.354 & 0.613 \\ 
\multicolumn{1}{c|}{} & 168 & \textbf{0.397} & \textbf{0.397} & \uline{0.402} & 0.419 & 0.64 \\ 
\multicolumn{1}{c|}{} & 336 & \textbf{0.424} & \textbf{0.424} & \uline{0.43} & 0.445 & 0.864 \\ 
\multicolumn{1}{c|}{} & 720 & \textbf{0.453} & \textbf{0.453} & \uline{0.457} & 0.487 & 0.993 \\ 
\hline
\multirow{5}*{\rotatebox{90}{Weather}} & 24 & \uline{0.088} & 0.09 & \uline{0.088} & \textbf{0.087} & 0.324 \\ 
\multicolumn{1}{c|}{} & 48 & \uline{0.114} & \uline{0.114} & 0.141 & \textbf{0.113} & 0.366 \\ 
\multicolumn{1}{c|}{} & 168 & \textbf{0.177} & \textbf{0.177} & \uline{0.178} & \uline{0.178} & 0.543 \\ 
\multicolumn{1}{c|}{} & 336 & \textbf{0.241} & \textbf{0.241} & \uline{0.244} & \uline{0.244} & 0.568 \\ 
\multicolumn{1}{c|}{} & 720 & \textbf{0.319} & \textbf{0.319} & 0.322 & \uline{0.321} & 0.601 \\ 
\hline
% &\multicolumn{3}{c|}{\makecell{\textbf{\citsm-Best} & \textbf{9.372}}	& \textbf{10.421} & \textbf{9.656} & \textbf{11.352} \\ \hline
\end{tabular}}
\caption{CI-\tsm-drill-down for self-supervised multivariate forecasting. MSE mean reported.}
\label{tab:ab_fm_1}
\end{table*}



\begin{table*}
\centering
\setlength{\tabcolsep}{2pt}
\scalebox{1.1}{
\begin{tabular}{c|c|c|c}
\hline  
& \makecell{FL} & \makecell{CI-\tsm\\-Best} & \makecell{Ts2Vec} \\
\hline
\multirow{5}*{ETTH1} & 24.0 & \textbf{0.314} & {0.599} \\ 
\multicolumn{1}{c|}{} & 48.0 & \textbf{0.343} & {0.629} \\ 
\multicolumn{1}{c|}{} & 168.0 & \textbf{0.397} & {0.755} \\ 
\multicolumn{1}{c|}{} & 336.0 & \textbf{0.424} & {0.907} \\ 
\multicolumn{1}{c|}{} & 720.0 & \textbf{0.453} & {1.048} \\ 
\hline 
\multirow{2}*{Electricity} & 336.0 & \textbf{0.16} & {0.349} \\ 
\multicolumn{1}{c|}{} & 720.0 & \textbf{0.187} & {0.375} \\ \hline
&\multicolumn{2}{c|}{\makecell{\textbf{\% Improvement}}}	& \textbf{50.7\%} \\ \hline

\end{tabular}}
\caption{CI-\tsm-Best vs Ts2Vec (MSE)}
\label{tab:ab_ts2vec}
\end{table*}

\section{Online Resources}
